# Supplementary material for: Recursive Visual Attention in Visual Dialog
Source: arXiv:1812.02664 source file (2019-04-06)
Supplement: Supplementary file 1 [file supp.tex]

\section*{Supplementary Material}

\input{section_supp/0-abstract}
\input{section_supp/1-network}
\input{section_supp/2-ablation}
